# Supplementary material for: Observation of higher-order topological states on a quantum computer
Source: arXiv:2303.02179 source file (2023-09-05)
Supplement: Supplementary file 1 [file supp.pdf]

# Observation of higher-order topological states on a quantum computer (supplementary information)

Jin Ming Koh,[1,*] Tommy Tai,[2,3,4,*] and Ching Hua Lee[4,†]

[1]*Division of Physics, Mathematics and Astronomy, Caltech, Pasadena, California 91125, US*
[2]*Department of Physics, MIT, Cambridge, Massachusetts 02142, US*
[3]*Cavendish Laboratory, University of Cambridge, JJ Thomson Ave, Cambridge CB3 0HE, UK*
[4]*Department of Physics, National University of Singapore, Singapore 117542*

* These authors contributed equally to this work.

† phylch@nus.edu.sg

**Square Lattice** ($d = 2$)

| Config. | $v^x_0$ | $v^x_1$ | $v^y_0$ | $v^y_1$ |
|---|---|---|---|---|
| C0 | 1.5 | 1.5 | 1.5 | −1.5 |
| C2 | 0.5 | 1.5 | 0.3 | −0.3 |
| C4 | 0.5 | 0.5 | 0.3 | −0.3 |
| | $w^x_0$ | $w^x_1$ | $w^y_0$ | $w^y_1$ |
| C0 | 0.5 | 0.5 | 0.5 | −0.5 |
| C2 | 1.5 | 0.5 | 1.7 | −1.7 |
| C4 | 1.5 | 1.5 | 1.7 | −1.7 |

**Cubic Lattice** ($d = 3$)

| Config. | $v^x_{00}$ | $v^x_{10}$ | $v^y_{00}$ | $v^y_{10}$ | $v^x_{01}$ | $v^x_{11}$ | $v^y_{01}$ | $v^y_{11}$ | $v^z_{01}$ | $v^z_{11}$ | $v^z_{10}$ | $v^z_{01}$ |
|---|---|---|---|---|---|---|---|---|---|---|---|---|
| C0 | 1.8 | 1.8 | 1.8 | −1.8 | 1.8 | 1.8 | −1.8 | 1.8 | −1.8 | 1.8 | 1.8 | −1.8 |
| C2a | 0.2 | 1.8 | 0.2 | −0.2 | 1.8 | 1.8 | −0.2 | 0.2 | −0.2 | 0.2 | 0.2 | −0.2 |
| C2b | 1.8 | 1.8 | 0.2 | −0.2 | 1.8 | 0.2 | −0.2 | 0.2 | −0.2 | 0.2 | 0.2 | −0.2 |
| C4a | 0.2 | 0.2 | 0.2 | −0.2 | 0.2 | 0.2 | −0.2 | 0.2 | −0.2 | 1.8 | 1.8 | −0.2 |
| C4b | 0.2 | 0.2 | 0.2 | −0.2 | 1.8 | 0.2 | −0.2 | 0.2 | −0.2 | 1.8 | 0.2 | −0.2 |
| C4c | 0.2 | 1.8 | 0.2 | −0.2 | 1.8 | 0.2 | −0.2 | 0.2 | −0.2 | 0.2 | 0.2 | −0.2 |
| C6 | 0.2 | 0.2 | 0.2 | −0.2 | 0.2 | 0.2 | −0.2 | 1.8 | −0.2 | 0.2 | 0.2 | −0.2 |
| C8 | 0.2 | 0.2 | 0.2 | −0.2 | 0.2 | 0.2 | −0.2 | 0.2 | −0.2 | 0.2 | 0.2 | −0.2 |
| | $w^x_{00}$ | $w^x_{10}$ | $w^y_{00}$ | $w^y_{10}$ | $w^x_{01}$ | $w^x_{11}$ | $w^y_{01}$ | $w^y_{11}$ | $w^z_{01}$ | $w^z_{11}$ | $w^z_{10}$ | $w^z_{01}$ |
| C0 | 0.2 | 0.2 | 0.2 | −0.2 | 0.2 | 0.2 | −0.2 | 0.2 | −0.2 | 0.2 | 0.2 | −0.2 |
| C2a | 1.8 | 0.2 | 1.8 | −1.8 | 0.2 | 0.2 | −1.8 | 1.8 | −1.8 | 1.8 | 1.8 | −1.8 |
| C2b | 0.2 | 0.2 | 1.8 | −1.8 | 0.2 | 1.8 | −1.8 | 1.8 | −1.8 | 1.8 | 1.8 | −1.8 |
| C4a | 1.8 | 1.8 | 1.8 | −1.8 | 1.8 | 1.8 | −1.8 | 1.8 | −1.8 | 0.2 | 0.2 | −1.8 |
| C4b | 1.8 | 1.8 | 1.8 | −1.8 | 0.2 | 1.8 | −1.8 | 1.8 | −1.8 | 0.2 | 1.8 | −1.8 |
| C4c | 1.8 | 0.2 | 1.8 | −1.8 | 0.2 | 1.8 | −1.8 | 1.8 | −1.8 | 1.8 | 1.8 | −1.8 |
| C6 | 1.8 | 1.8 | 1.8 | −1.8 | 1.8 | 1.8 | −1.8 | 0.2 | −1.8 | 1.8 | 1.8 | −1.8 |
| C8 | 1.8 | 1.8 | 1.8 | −1.8 | 1.8 | 1.8 | −1.8 | 1.8 | −1.8 | 1.8 | 1.8 | −1.8 |

**Tesseract Lattice** ($d = 4$)

| Config. | $v^x_{000}$ | $v^x_{100}$ | $v^y_{000}$ | $v^y_{100}$ | $v^x_{010}$ | $v^x_{110}$ | $v^y_{010}$ | $v^y_{110}$ | $v^z_{010}$ | $v^z_{110}$ | $v^z_{100}$ | $v^z_{010}$ | $v^x_{001}$ | $v^x_{101}$ | $v^x_{011}$ | $v^x_{111}$ |
|---|---|---|---|---|---|---|---|---|---|---|---|---|---|---|---|---|
| C0 | 1.8 | 1.8 | 1.8 | −1.8 | −1.8 | 1.8 | 1.8 | 1.8 | 1.8 | 1.8 | 1.8 | −1.8 | 1.8 | −1.8 | 1.8 | 1.8 |
| C2 | 0.2 | 0.2 | 0.2 | −0.2 | −0.2 | 0.2 | 0.2 | 0.2 | 0.2 | 0.2 | 0.2 | −0.2 | 0.2 | −0.2 | 0.2 | 0.2 |
| C4 | 0.2 | 0.2 | 0.2 | −0.2 | −0.2 | 0.2 | 0.2 | 0.2 | 0.2 | 1.8 | 1.8 | −0.2 | 0.2 | −0.2 | 0.2 | 0.2 |
| C8 | 0.2 | 0.2 | 0.2 | −0.2 | −0.2 | 0.2 | 0.2 | 0.2 | 0.2 | 0.2 | 0.2 | −0.2 | 0.2 | −0.2 | 0.2 | 0.2 |
| C16 | 0.2 | 0.2 | 0.2 | −0.2 | −0.2 | 0.2 | 0.2 | 0.2 | 0.2 | 0.2 | 0.2 | −0.2 | 0.2 | −0.2 | 0.2 | 0.2 |
| E | 0 | 2.5 | 0.5 | 0 | 0 | 0.5 | 2.5 | 0.5 | 0.5 | 0 | 2.5 | 0 | 0.5 | 0 | 2.5 | 0 |
| | $w^x_{000}$ | $w^x_{100}$ | $w^y_{000}$ | $w^y_{100}$ | $w^x_{010}$ | $w^x_{110}$ | $w^y_{010}$ | $w^y_{110}$ | $w^z_{010}$ | $w^z_{110}$ | $w^z_{100}$ | $w^z_{010}$ | $w^x_{001}$ | $w^x_{101}$ | $w^x_{011}$ | $w^x_{111}$ |
| C0 | 0.2 | 0.2 | 0.2 | −0.2 | −0.2 | 0.2 | 0.2 | 0.2 | 0.2 | 0.2 | 0.2 | −0.2 | 0.2 | −0.2 | 0.2 | 0.2 |
| C2 | 1.8 | 1.8 | 1.8 | −1.8 | −1.8 | 1.8 | 1.8 | 1.8 | 1.8 | 1.8 | 1.8 | −1.8 | 1.8 | −1.8 | 1.8 | 1.8 |
| C4 | 1.8 | 1.8 | 1.8 | −1.8 | −1.8 | 1.8 | 1.8 | 1.8 | 1.8 | 0.2 | 0.2 | −1.8 | 1.8 | −1.8 | 1.8 | 1.8 |
| C8 | 1.8 | 1.8 | 1.8 | −1.8 | −1.8 | 1.8 | 1.8 | 1.8 | 1.8 | 1.8 | 1.8 | −1.8 | 1.8 | −1.8 | 1.8 | 1.8 |
| C16 | 1.8 | 1.8 | 1.8 | −1.8 | −1.8 | 1.8 | 1.8 | 1.8 | 1.8 | 1.8 | 1.8 | −1.8 | 1.8 | −1.8 | 1.8 | 1.8 |
| E | 2 | −0.5 | 1.5 | −2 | −2 | 1.5 | −0.5 | 1.5 | 1.5 | 2 | −0.5 | −2 | 1.5 | −2 | −0.5 | 2 |

| Config. | $v^y_{001}$ | $v^y_{101}$ | $v^y_{011}$ | $v^y_{111}$ | $v^z_{001}$ | $v^z_{101}$ | $v^z_{011}$ | $v^z_{111}$ | $v^w_{000}$ | $v^w_{100}$ | $v^w_{010}$ | $v^w_{110}$ | $v^w_{001}$ | $v^w_{101}$ | $v^w_{011}$ | $v^w_{111}$ |
|---|---|---|---|---|---|---|---|---|---|---|---|---|---|---|---|---|
| C0 | 1.8 | 1.8 | −1.8 | 1.8 | 1.8 | −1.8 | 1.8 | 1.8 | −1.8 | 1.8 | 1.8 | 1.8 | 1.8 | 1.8 | 1.8 | −1.8 |
| C2 | 0.2 | 0.2 | −0.2 | 0.2 | 0.2 | −0.2 | 0.2 | 0.2 | −0.2 | 1.8 | 1.8 | 1.8 | 1.8 | 1.8 | 1.8 | −1.8 |
| C4 | 0.2 | 0.2 | −0.2 | 0.2 | 0.2 | −1.8 | 0.2 | 1.8 | −0.2 | 0.2 | 0.2 | 1.8 | 1.8 | 1.8 | 1.8 | −1.8 |
| C8 | 0.2 | 0.2 | −0.2 | 0.2 | 0.2 | −0.2 | 0.2 | 0.2 | −0.2 | 0.2 | 0.2 | 0.2 | 1.8 | 1.8 | 1.8 | −1.8 |
| C16 | 0.2 | 0.2 | −0.2 | 0.2 | 0.2 | −0.2 | 0.2 | 0.2 | −0.2 | 0.2 | 0.2 | 0.2 | 0.2 | 0.2 | 0.2 | −0.2 |
| E | 0.5 | 2.5 | 0 | 0.5 | 0 | 0 | 2.5 | 0.5 | 0 | 0.5 | 0.5 | 0.5 | 0.5 | 0.5 | 0.5 | 0 |
| | $w^y_{001}$ | $w^y_{101}$ | $w^y_{011}$ | $w^y_{111}$ | $w^z_{001}$ | $w^z_{101}$ | $w^z_{011}$ | $w^z_{111}$ | $w^w_{000}$ | $w^w_{100}$ | $w^w_{010}$ | $w^w_{110}$ | $w^w_{001}$ | $w^w_{101}$ | $w^w_{011}$ | $w^w_{111}$ |
| C0 | 0.2 | 0.2 | −0.2 | 0.2 | 0.2 | −0.2 | 0.2 | 0.2 | −0.2 | 0.2 | 0.2 | 0.2 | 0.2 | 0.2 | 0.2 | −0.2 |
| C2 | 1.8 | 1.8 | −1.8 | 1.8 | 1.8 | −1.8 | 1.8 | 1.8 | −1.8 | 0.2 | 0.2 | 0.2 | 0.2 | 0.2 | 0.2 | −0.2 |
| C4 | 1.8 | 1.8 | −1.8 | 1.8 | 1.8 | −0.2 | 1.8 | 0.2 | −1.8 | 1.8 | 1.8 | 0.2 | 0.2 | 0.2 | 0.2 | −0.2 |
| C8 | 1.8 | 1.8 | −1.8 | 1.8 | 1.8 | −1.8 | 1.8 | 1.8 | −1.8 | 1.8 | 1.8 | 1.8 | 0.2 | 0.2 | 0.2 | −0.2 |
| C16 | 1.8 | 1.8 | −1.8 | 1.8 | 1.8 | −1.8 | 1.8 | 1.8 | −1.8 | 1.8 | 1.8 | 1.8 | 1.8 | 1.8 | 1.8 | −1.8 |
| E | 1.5 | −0.5 | −2 | 1.5 | 2 | −2 | −0.5 | 1.5 | −2 | 1.5 | 1.5 | 1.5 | 1.5 | 1.5 | 1.5 | −2 |

Supplementary Table 1. Values of intra- and inter-cell hopping coefficients, respectively $v^{\alpha}_{\boldsymbol{\pi}(\mathbf{r}_\alpha)}$ and $w^{\alpha}_{\boldsymbol{\pi}(\mathbf{r}_\alpha)}$ along direction $\alpha \in \{x, y, z, w\}$ and at parity $\boldsymbol{\pi}(\mathbf{r}_\alpha)$ on the remaining axes, used in simulations of the square, cubic, and tesseract HOT lattices. Numerical values are explicitly listed for clarity; a systematic procedure to assign coefficients for corner-mode configurations on square and cubic lattices is available in Ref. [1], generalizable to higher dimensions.

| Lattice | Configuration | Initial States $\|\psi\rangle$ |
|---|---|---|
| Square ($d=2$) | C2 | $\left(\|1,1\rangle \pm \|L,1\rangle\right)/\sqrt{2}$ |
| | C4 | $\left(\|1,1\rangle \pm \|L,1\rangle\right)/\sqrt{2}$ |
| | | $\left(\|1,L\rangle \pm \|L,L\rangle\right)/\sqrt{2}$ |
| Cubic ($d=3$) | C4a | $\left(\|1,1,1\rangle \pm \|1,1,L\rangle + \|1,L,L\rangle\right)/\sqrt{3}$ |
| | | $\left(\|1,1,1\rangle \pm \|1,L,1\rangle - \|1,L,L\rangle\right)/\sqrt{3}$ |
| | C4b | $\left(\|1,1,1\rangle \pm \|1,L,1\rangle - \|1,L,L\rangle\right)/\sqrt{3}$ |
| | | $\left(\|1,1,1\rangle + \|1,L,L\rangle \pm \|L,1,1\rangle\right)/\sqrt{3}$ |
| | C8 | $\left(\|1,1,1\rangle \pm \|1,L,1\rangle \pm \|L,1,1\rangle\right)/\sqrt{3}$ |
| | | $\left(\|1,1,L\rangle \pm \|1,L,L\rangle \pm \|L,1,L\rangle\right)/\sqrt{3}$ |
| | | $\left(\|1,L,1\rangle - \|L,1,1\rangle \pm \|L,L,1\rangle\right)/\sqrt{3}$ |
| | | $\left(\|1,L,L\rangle + \|L,L,1\rangle \pm \|L,L,L\rangle\right)/\sqrt{3}$ |

Supplementary Table 2. Initial states used in IQPE to probe the existence of corner HOT modes, which are constructed as simple superpositions of corner-localized states. Above, a state of form $|x,y\rangle$ is perfectly localized on the site at spatial coordinates $(x,y)$, and likewise in the three-dimensional case. Lattices are of side length $L$.

[1] L. Li, M. Umer, and J. Gong, Direct prediction of corner state configurations from edge winding numbers in two- and three-dimensional chiral-symmetric lattice systems, Phys. Rev. B **98**, 205422 (2018).
